# Supplementary material for: Rare Gems: Finding Lottery Tickets at Initialization
Source: arXiv:2202.12002 source file (2022-06-02)
Supplement: Supplementary file 1 [file AppendixB.tex]

\section{Theoretical Results and Proofs}
Let $f(\vx): \mathbb{R}^{d_0} \rightarrow \mathbb{R}$ be the target FC network with $l$ layers and ReLU activations, represented as
\begin{equation*}
    f(\vx) = \sigma(\mW_l\sigma(\mW_{l-1} \dots \sigma(\mW_1\vx))),
\end{equation*}
where $\vx \in \mathbb{R}^{d_0}$ is the input, $\sigma(\vz) = \max\{\vz, 0\}$ is the ReLU activation and $\mW_i \in \mathbb{R}^{d_{i} \times d_{i-1}}$ is the weight matrix of layer $i \in [l]$. For simplicity assume that $d_i = d\; \forall i \in [l]$. Let $\mathcal{D}(\vx, y)$ be some data distribution where $y \in \mathbb{R}$ is the target. Let $\ell(y, \hat{y})$ be an $L-$lipschitz loss function. We say that $f(\vx)$ is $\epsilon-$accurate with respect to $\ell(\cdot)$ if
\begin{equation*}
    \mathbb{E}_{(x, y) \sim \mathcal{D}} \ell(y, f(x)) \leq \epsilon
\end{equation*}
We say that a network $f(\vx)$ is $k-$sparse if the number of non-zero activations in any layer is atmost $k$. More precisely, for any layer $i \in [l]$, $\sigma(W_{i}\sigma(W_{i-1}\dots \sigma(W_i(\vx)))$ is a $k$-sparse vector for any $\vx \in \mathbb{R}^{d_0}$.

\begin{corollary}
Let $f(\vx)$ be an FC ReLU network of width $d$ and depth $l$ which is $\epsilon-$accurate with respect to some lipschitz loss function $\ell$. Suppose $f(\vx)$ is sparse in the sense that every layer only has $o(d^{1-\gamma})$ non-zero activations for some $\gamma > 0$. Then, one can prune a randomly initialized FC ReLU network $g(x)$ of width $O(d)$ and depth $2l$ so that the subnetwork is $O(\epsilon + d^{-\alpha})-$accurate with respect to $\ell$ for any $\alpha > 1$.
\end{corollary}

\begin{proof}
Rough Proof sketch:
Need to re-create the proof from \cite{pensia2020optimal} for the layer approximation. Because of the weight re-use trick, if the number of activations per layer is $o(d^{1-\gamma})$, then the new network only needs to be $O(d^{1-\gamma} \cdot \log(dl/\beta))$ wide if we want to be $\beta-$close to $f$ \ie if we prune a network $g(\vx)$ which is $O(d^{1-\gamma} \log(dl/\beta))$ wide and $2l$ deep then
\begin{equation*}
    \lVert f(\vx) - \tilde{g(\vx)}\rVert \leq \beta
\end{equation*}
Since $\ell$ is $L-$lipschitz, we have that
\begin{align*}
    \lVert \ell(y, f(\vx) - \ell(y, \tilde{g(\vx)}) \rVert \leq L\cdot \lVert f(\vx) - \tilde{g(\vx)}\rVert \leq L\beta
\end{align*}
Since $f$ is $\epsilon-$accurate w.r.t $\ell$,
\begin{align*}
    \mathbb{E}_{x, y \sim \mathcal{D}} \ell(y, \tilde{g}(\vx)) &= \mathbb{E}_{x, y \sim \mathcal{D}} \left[(\ell(y, \tilde{g}(\vx)) - \ell(y, f(\vx)\right] + \mathbb{E}_{x, y \sim \mathcal{D}} \left[(\ell(y, f(\vx))\right]\\
    &\leq \mathbb{E}_{x, y \sim \mathcal{D}} L\beta + \epsilon\\
    &\leq L\beta + \epsilon
\end{align*}
Choosing $\beta = d^{-\alpha}/L$ for any $\alpha > 1$ gives us that $\mathbb{E}_{x, y \sim \mathcal{D}} \ell(y, \tilde{g}(\vx)) = O(\epsilon + d^{-\alpha}$ and that $g$ is $O(d^{1-\gamma}\log(d^{\alpha+1}l) = O(d)$ wide.

\ks{I don't want to repeat Ankit and Shashank's proof completely but I think that's the only way to be rigorous.}

\end{proof}

\begin{algorithm}[t]
\DontPrintSemicolon
\SetNoFillComment
\caption{\algo{} algorithm}\label{Algo:GM}
\KwIn{Dataset $D = \{(\vx_i, y_i)\}$, step size $\eta$, rounding function $r(\cdot)$, number of epochs $E$, pruning period $T$, prune rate $k \in [0,1]$}
\KwOut{Mask $\vm \in \{0,1\}^d$}
$\vw \gets$ random vector in $\mathbb{R}^d$\;
$\vp \gets$ random vector in $[0,1]^d$\;
$\vq \leftarrow \mathbf{1}_d$\;
\For{$j$ in $1,2,\dots, E$}{
    \For{$(\vx_i, y_i) \in D$}{
      $\vw_{\op{eff}} \gets (\vw \odot \vq) \odot r(\vp)$\;
      \tcc{Use STE to compute $\nabla(r)$}
      $\vp \gets \vp - \eta \nabla_{\vp}\  \ell( f(\vw_{\op{eff}}; \vx_i), y_i)$\;
      $\vp \gets \op{proj}_{[0,1]^d} \vp$\;
    }
    \uIf{$\mathrm{mod} (j, T) = 0$}{
        $p_{\op{thresh}} \gets$ bottom-k fraction in $\vp \odot \vq$\;
        $\vq \gets \vq \odot \mathds{1}_{\vp \geq p_{\op{thresh}}}$\;
      }
    }
$\vm \gets r(\vp) \odot \vq$
\end{algorithm}
